# Supplementary material for: Scaling of Rayleigh-Taylor mixing in porous media
Source: arXiv:2006.07175 source file (2020-06-12)
Supplement: Supplementary file 1 [file supmat.pdf]

# Supplemental Material to
# Scaling of Rayleigh-Taylor mixing in porous media

G. Boffetta, M. Borgnino, and S. Musacchio
*Dipartimento di Fisica and INFN, Università di Torino, via P. Giuria 1, 10125 Torino, Italy*

## I. LINEAR STABILITY OF A PIECEWISE-LINEAR PROFILE

Linear stability analysis of the miscible RT problem in porous media has been studied by several authors starting from [1]. Here we follow the method discussed in [2] simplified to the case of a single solute. We consider a quasi-stationary density profile $\rho_0(z)$ which, together with $\mathbf{u}_0 = 0$ represents our basic state, while the perturbations are written as $\rho_1(z)$ and $\mathbf{u}_1$. By linearizing the two-dimensional version of the Darcy-Boussinesq equations around the basic state we obtain the equations for the perturbations

$$\psi_1 = \frac{\kappa g}{\mu\phi}\partial_x \rho_1 \tag{1}$$

$$\partial_t \rho_1 - (\partial_x \psi_1)(\partial_z \rho_0) = D\nabla^2 \rho_1 \tag{2}$$

where $\psi_1$ represents the perturbed stream function. By looking for a solution to (1-2) in the form $\rho_1(\mathbf{x}, t) = e^{\gamma t + ikx}\hat{\rho}_1(z)$ with the appropriate boundary conditions in $z$, one in principle ends up with the dispersion relation for the growth rate $\gamma(k)$. In the case of a step density jump, $\rho_0(z) = \Delta\rho[\theta(z) - 1/2]$ one has the explicit expression for the dispersion relation [2]

$$\gamma = \frac{k}{2}\left[w_0 - Dk - \sqrt{Dk(2w_0 + Dk)}\right] \tag{3}$$

with $w_0 = \Delta\rho\kappa g/(\mu\phi)$. From (3) one sees that unstable modes have a cut-off at wavenumber $k_c = \frac{w_0}{4D}$ and that the grow rate is maximum for $k = \frac{\sqrt{5}-2}{2D}w_0$.

We performed a set of numerical simulations of the two-dimensional linear model (1-2) for a piecewise-linear basic state with $\rho_0(z) = -1/2$ for $z < z_1$, $\rho_0(z) = +1/2$ for $z > z_1$ and $\rho(z) = z/(2z_1)$ for $|z| \leq z_1$ (i.e. with a density jump $\Delta\rho = 1$) as a good approximation of the mean density profile observed in the development of the mixing layer (see Fig.2A in the manuscript). We have measured the rate of exponential growth of each wavenumber to obtain the numerical dispersion relation $\sigma(k)$. In the limit $z_1 \to 0$ one recovers the RT initial condition with the corresponding dispersion relation (3). The results are shown in Fig. 1 together with the prediction (3). While the growth rates of the case with the steepest profile ($z_1 = \delta z$) are close to those of the step profile (3), we find that the stability of the piecewise-linear density profile increases at increasing $z_1$.

The dispersion relation (3) has also been used to validate the full 3D numerical code. In this case, the initial condition for the density is a regularized step profile modulated by a monochromatic wave: $\rho(\mathbf{x}, 0) = \frac{1}{2}\tanh\left(\frac{z-h(x)}{\lambda}\right)$ with $h(x) = \varepsilon\sin(kx)$. The amplitude of the wave is very small, $\varepsilon k \ll 1$, but larger than the width of the interface $\varepsilon > \lambda$. In order to resolve the discontinuity at the interface, we chose $\lambda \simeq 8\Delta x$. The three-dimensional Darcy-Boussinesq equations are integrated for a short time and the growth rate $\gamma$ is evaluated by an exponential fit of the time evolution of the square vertical velocity [3]. The measured values of the growth rates coincide with the corresponding theoretical values given by Eq.(3). The results for $k = 1$ and $k = 2$ are shown in Fig. 1.

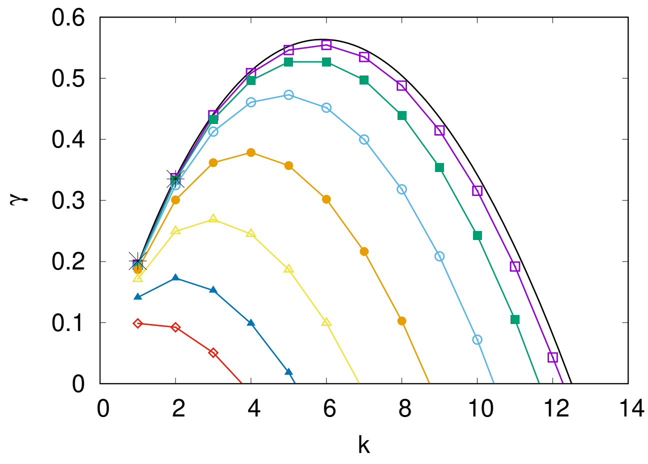


FIG. 1. Numerical and analytical dispersion relation for the piecewise-linear basic state. The solid black line represents the analytical expression (3) for a step profile ($z_1 \to 0$). Lines with symbols are the results from numerical simulations of (1-2) at resolution $M = 256$ with $w_0 = 0.5$ and $D = 10^{-2}$, with different $z_1$, starting from $z_1 = \delta z$ (open squares), $z_1 = 2\delta z$ (filled squares), $z_1 = 4\delta z$ (open circles), $z_1 = 8\delta z$ (filled circles), $z_1 = 16\delta z$ (open triangles), $z_1 = 32\delta z$ (filled triangles), $z_1 = 64\delta z$ (open diamonds). The grid spacing is $\delta z = L/M$ with $L = 2\pi$. The two black asterisk are the validation of the full 3D model for $k = 1$ and $k = 2$.

[1] R A Wooding, "The Stability of an Interface Between Miscible Fluids in a Porous Medium," J. Applied Math. Phys. (ZAMP) **13**, 255 (1962).

[2] P M J Trevelyan, C Almarcha, and A De Wit, "Buoyancy-driven instabilities of miscible two-layer stratifications in porous media and Hele-Shaw cells," J. Fluid Mech. **670**, 38 (2011).

[3] Antonio Celani, Andrea Mazzino, Paolo Muratore-Ginanneschi, and Lara Vozella, "Phase-field model for the Rayleigh–Taylor instability of immiscible fluids," J. Fluid Mech. **622**, 115–134 (2009).
